# Supplementary material for: Solving Boltzmann equation with neural sparse representation
Source: arXiv:2302.09233 source file (2023-02-18)
Supplement: Supplementary file 1 [file article_appendix.tex]

\appendix 

\section{Appendix}

% \subsection{Fast Fourier method}

\subsection{Grad method and low rank}

\begin{remark}
In the framework of Hermite spectral method \cite{wang2019approximation}, and Grad's moment method \cite{grad1949kinetic} to solve Boltzmann equation, the approximation to the distribution function with a series of basis functions can be rewritten into the form of CPD, and we omit the proof here. 

In the $M$-th order Grad moments method, the distribution function is assumed to be

\begin{equation}
f(\bm x,\bm v,t)= \mathcal{M}^{[\bm u( \bm x,t),T(\bm x,t)]}(\bm v) \sum_{|\alpha|\leq M} f_{\alpha}(\bm x,t) \mathcal{H}_{\alpha}^{[u(\bm x,t),T(\bm x,t)]}(\bm v)
\end{equation}

\begin{equation}
f(\bm v)= \mathcal{M}(\bm v) \sum_{|\alpha'|\leq M} f_{\alpha'}\mathcal{H}_{\alpha'}(\bm v) 
\end{equation}

$$
\mathcal{H}_{\alpha'}(\bm v)=v_1^{\alpha'_1}v_2^{\alpha'_2}v_3^{\alpha'_3}
$$

\begin{equation}
f(\bm v)= \sum_{|\alpha'|\leq M} f_{\alpha'} v_1^{\alpha'_1}v_2^{\alpha'_2}v_3^{\alpha'_3} \mathcal{M}_1(v_1)\mathcal{M}_2(v_2)\mathcal{M}_3(v_3)
\end{equation}

\end{remark}

\label{app:fft}
